# Supplementary material for: Unconditional Priors Matter! Improving Conditional Generation of Fine-Tuned Diffusion Models
Source: arXiv:2503.20240 source file (2026-02-10)
Supplement: Supplementary file 1 [file 011IP2P_CFG++.tex]

\section{InstructPix2Pix CFG++} \label{sec:ip2p-cfg++}
We find that using CFG++ for IP2P either does not edit the image or fails to consistently generate plausible images, and thus only include CFG results in the main text. However, our method of replacing the unconditional noise in the CFG++ formulation with the \emph{base model} unconditional noise does generate plausible edits. We hypothesize that the failure of CFG++ on IP2P is due to the low quality of the unconditional noise which is exacerbated by the added complexity of the dual CFG formulation. As shown in Fig.~\ref{fig:ip2p-qualitatives-cfg++}, replacing the unconditional noise with the unconditional noise from \texttt{SD1.5} or \texttt{SD2.1} results in coherent edits. 

Quantitative results are also shown in Tab.~\ref{tab:ip2p-results-cfg++}. While CFG++ with IP2P fails, our method using the CFG++ formulation yields competitive results with our method using the CFG formulation (Tab.~\ref{tab:ip2p-results} \refinpaper{}).

\begin{table}
    \begin{minipage}{\linewidth}
    \centering
    \scriptsize
        % \begin{tabularx}{\linewidth}{c | Y | Y | Y | Y | Y}
        \begin{tabularx}{\linewidth}{>{\centering\arraybackslash}m{0.175\textwidth} | >{\centering\arraybackslash}m{0.12\textwidth} | >{\centering\arraybackslash}m{0.12\textwidth} | >{\centering\arraybackslash}m{0.11\textwidth} | >{\centering\arraybackslash}m{0.09\textwidth} | > {\centering\arraybackslash}m{0.09\textwidth}}
        \toprule
         Method & CLIP-I $\uparrow$ & CLIP-T $\uparrow$ & \makecell{CLIP-D $\uparrow$} & \makecell{IR $\uparrow$} & PS $\uparrow$ \\
        \midrule
        IP2P (CFG++) & 0.780 & 0.202 & 0.116 & -2.025 & 0.142 \\
        w/ SD1.5 & \underline{0.919} & \underline{0.294} & \textbf{0.158} & \textbf{-0.406} & \textbf{0.490} \\
        w/ SD2.1 & \textbf{0.922} & \textbf{0.295} & \underline{0.157} & \underline{-0.436} & \textbf{0.490} \\
        \bottomrule
        \end{tabularx}
        \vspace{-0.5\baselineskip}
        \caption{\textbf{Image Editing with InstructPix2Pix (IP2P)~\cite{brooks2023instructpix2pix} using the CFG++ formulation.} We normalize text and image similarity scores: CLIP-I, CLIP-T, and CLIP-D. The PickScore (PS) baseline is IP2P \emph{CFG} which is shown in Tab.~\ref{tab:ip2p-results} \refinpaper{}.
        (\textbf{bold} represents the best, and \underline{underline} represents the second best method.)}
        \vspace{-\baselineskip}
    \label{tab:ip2p-results-cfg++}
    \end{minipage}
\end{table}
