# Supplementary material for: Unconditional Priors Matter! Improving Conditional Generation of Fine-Tuned Diffusion Models
Source: arXiv:2503.20240 source file (2026-02-10)
Supplement: Supplementary file 2 [file 012TweediesDerivation.tex]

\section{Derivation of CFG Tweedies} \label{sec:derivation-cfg-tweedies}
We provide details on the derivation of the CFG Tweedies $\V{x}_{0|t}^{(\gamma)}$ shown in Eq.~\ref{eq:cfg-tweedies-interpretation} in Sec.~\ref{sec:cfg-tweedies-guidance} \refofpaper{}:
\vspace*{-0.8\baselineskip}
\begin{align*}
    \V{x}_{0|t}^{(\gamma)} 
    &= \frac{1}{\sqrt{\bar{\alpha}_t}} \left( \V{x}_t - \sqrt{1 - \bar{\alpha}_t} \epsilon_\theta^{(\gamma)}(\V{x}_t, c) \right) \\
    &= \frac{1}{\sqrt{\bar{\alpha}_t}} \left( \V{x}_t - \sqrt{1 - \bar{\alpha}_t} ((1 - \gamma) \epsilon_\theta(\V{x}_t, \emptyset) + \gamma \epsilon_\theta(\V{x}_t, c)) \right) \\
    &= (1 - \gamma) \frac{1}{\sqrt{\bar{\alpha}_t}} \left( \V{x}_t - \sqrt{1 - \bar{\alpha}_t} \epsilon_\theta(\V{x}_t,\emptyset) \right) \\
    & \qquad + \gamma \frac{1}{\sqrt{\bar{\alpha}_t}} \left( \V{x}_t - \sqrt{1 - \bar{\alpha}_t} \epsilon_\theta(\V{x}_t,c) \right) \\
    &= (1-\gamma) \V{x}_{0|t}^\emptyset + \gamma \V{x}_{0|t}^c
\end{align*}
