# Supplementary material for: Unconditional Priors Matter! Improving Conditional Generation of Fine-Tuned Diffusion Models
Source: arXiv:2503.20240 source file (2026-02-10)
Supplement: Supplementary file 3 [file 013VDM.tex]

\section{DynamiCrafter~\cite{xing2025dynamicrafter}} \label{sec:dynamicrafter}
In this section, we report results from applying our method to DynamiCrafter~\cite{xing2025dynamicrafter}, an image-to-video diffusion model fine-tuned from the text-to-video diffusion model VideoCrafterT2V~\cite{chen2023videocrafter1}. DynamiCrafter incorporates the dual text-image CFG formulation shown in Eq.~\ref{eq:ip2p-dual-cfg} like InstructPix2Pix~\cite{brooks2023instructpix2pix}. For our method, we replace the DynamiCrafter fully unconditional noise with the VideoCrafterT2V unconditional noise. We sample $256 \times 256$ resolution videos using 50 steps of DDIM with a CFG scale of $\gamma_T = 7.5$ and $\gamma_I = 1.5$. Although the original paper uses a CFG scale of $\gamma_T = \gamma_I = 7.5$, we find that this choice of CFG scale results in mostly static images, as shown in their low dynamic degree of 40.57\% in the VBench benchmark~\cite{huang2024vbench}. In contrast, the baseline DynamiCrafter with our choice of CFG scale has a higher dynamic degree of 59.59\%. We report quantitative results using VBenchI2V~\cite{huang2024vbench, huang2023vbenchgithub} which measures video quality and video-condition consistency across multiple dimensions. For more details on the metrics, please refer to the VBench paper~\cite{huang2024vbench}. Quantitative results are reported in Tab.~\ref{tab:dynamicrafter-results}. All metrics are scored out of 100, with higher scores indicating better performance. Our method outperforms the baseline in 7 out of 9 metrics. In particular, our method yields more consistent video generation with higher aesthetic quality. As shown in Fig.~\ref{fig:dynamicrafter-qualitatives}, our method is more temporally consistent (first two videos) and less distorted (last video). 

\input{tables/DynamiCrafter_results}
\input{figures/dynamicrafter_qualitatives}
